# Supplementary material for: Thermal Pure Quantum Matrix Product States Recovering a Volume Law Entanglement
Source: arXiv:2005.06829 source file (2021-05-28)
Supplement: Supplementary file 1 [file supple_mpstpq.pdf]

# Supplementary Material for "Thermal Pure Quantum Matrix Product States Recovering a Volume Law Entanglement"

Atsushi Iwaki,[1] Akira Shimizu,[1,2] and Chisa Hotta[1]

[1]*Department of Basic Science, The University of Tokyo, 3-8-1 Komaba, Meguro, Tokyo 153-8902, Japan*
[2]*Komaba Institute for Science, The University of Tokyo, 3-8-1 Komaba, Meguro, Tokyo 153-8902, Japan*
(Dated: November 24, 2020)

After giving a brief review of important properties of various quantum states that represent a thermal equilibrium state, we derive Eq. (2) in the main text.

*Various quantum states representing the same thermal equilibrium state.*
Consider a thermal equilibrium state specified by energy $E$ and size $N$, which has an inverse temperature $\beta$. Here, we omit some other possible additional variables that may also be necessary to specify the equilibrium state. The equilibrium state is uniquely determined in thermodynamics. Whereas in statistical mechanics, there are various quantum-mechanical representations, such as the microcanonical density operator $\hat{\rho}(E,N)$, the canonical density operator $\hat{\rho}(\beta,N)$[1], and the microcanonical TPQ state $|k,N\rangle$ where the parameter $k$ is taken such that $\langle\hat{H}\rangle = E$, and the canonical TPQ state $|\beta,N\rangle$. In the thermodynamic limit, all these states give the same expectation value for any low-order polynomial of local observables. For example, for a single-site operator $\hat{\mathcal{O}}_1$, we find the following;

$$\mathrm{Tr}\left[\hat{\rho}(E,N)\hat{\mathcal{O}}_1\right] + o(N^0) = \mathrm{Tr}\left[\hat{\rho}(\beta,N)\hat{\mathcal{O}}_1\right] + o(N^0) = \langle E_k,N|\hat{\mathcal{O}}_1|E_k,N\rangle + o(N^0) = \langle\beta,N|\hat{\mathcal{O}}_1|\beta,N\rangle + o(N^0). \tag{S1}$$

In this context, any of these states can equally represent the equilibrium state. These quantum states give the thermodynamic functions as the logarithms of their normalization factors. Such thermodynamic functions are equivalent in the sense that any one of them can be obtained from the other one through the Legendre transform or its generalization [2], and is referred to as 'equivalence of ensembles' for the case of Gibbs ensembles.

*Von Neumann entropy.*
While the Gibbs states, $\hat{\rho}(E,N)$ and $\hat{\rho}(\beta,N)$, or the TPQ states, $|k,N\rangle$ and $|\beta,N\rangle$, yield the same *thermodynamic quantities*, their von Neumann entropy $S_{\mathrm{vN}}$, which are not thermodynamic quantities, are different from each other. In fact, we find

$$S_{\mathrm{vN}}(\hat{\rho}(E,N)) + o(N) = S_{\mathrm{vN}}(\hat{\rho}(\beta,N)) + o(N) = S_{\mathrm{th}}(\beta,N), \tag{S2}$$

where $S_{\mathrm{th}}(E,N)$ is the thermodynamics entropy, whereas

$$S_{\mathrm{vN}}(|k,N\rangle\langle k,N|) = S_{\mathrm{vN}}(|\beta,N\rangle\langle\beta,N|) = 0. \tag{S3}$$

These relationships hold for the von Neumann entropy of the total system of size $N$.

Let us now turn to the $S_{\mathrm{vN}}$ of the subsystem of size $n$, given as

$$S_{\mathrm{vN}}(\hat{\rho}_n) = -\,\mathrm{Tr}[\hat{\rho}_n \ln \hat{\rho}_n]. \tag{S4}$$

Here $\hat{\rho}_n$ denotes the reduced density operator of either one of the Gibbs and the TPQ states. Now, one can regard the total system as an assembly of $N/n$ subsystems (unit cells) of size $n$, and consider a local operator $\hat{\mathcal{O}}_1^{\mathrm{new}}$ acting on the unit cell. The unit cell is a "single site" of a system of total size $N/n$, and thus we find

$$\begin{aligned}&\mathrm{Tr}\left[\hat{\rho}(E,N)\hat{\mathcal{O}}_1^{\mathrm{new}}\right] + o((N/n)^0) = \mathrm{Tr}\left[\hat{\rho}(\beta,N)\hat{\mathcal{O}}_1^{\mathrm{new}}\right] + o((N/n)^0)\\ &= \langle E,N|\hat{\mathcal{O}}_1^{\mathrm{new}}|E,N\rangle + o((N/n)^0) = \langle\beta,N|\hat{\mathcal{O}}_1^{\mathrm{new}}|\beta,N\rangle + o((N/n)^0).\end{aligned} \tag{S5}$$

At the same time, $\hat{\mathcal{O}}_1^{\mathrm{new}}$ is an $n$-site observable $\mathcal{O}_n$ acting on $n$-sites of the size-$N$ system, hence Eq. (S5) is rewritten as

$$\begin{aligned}&\mathrm{Tr}\left[\hat{\rho}(E,N)\hat{\mathcal{O}}_n\right] + o((N/n)^0) = \mathrm{Tr}\left[\hat{\rho}(\beta,N)\hat{\mathcal{O}}_n\right] + o((N/n)^0)\\ &= \langle E,N|\hat{\mathcal{O}}_n|E,N\rangle + o((N/n)^0) = \langle\beta,N|\hat{\mathcal{O}}_n|\beta,N\rangle + o((N/n)^0).\end{aligned} \tag{S6}$$

This means that the reduced density operator $\hat{\rho}_n$ is identical for all these states except for the small difference of $o((N/n)^0)$.

On the other hand, we can easily show that, when $1 \ll n \ll N$[3], $\hat{\rho}_n$ of $\hat{\rho}(E, N)$ is the canonical Gibbs state of size-$n$[4], following the standard argument for the derivation of the canonical ensemble from the microcanonical ensemble of a larger systetem. Hence, we find

$$S_{\mathrm{vN}}(\hat{\rho}_n)/n = S_{\mathrm{vN}}(\hat{\rho}(\beta, n))/n + o(n^0) + o((N/n)^0) \tag{S7}$$

*for all Gibbs and TPQ states.* Furthermore, as in the case of Eq. (S2), we have

$$S_{\mathrm{vN}}(\hat{\rho}(\beta, n)) + o(n) = S_{\mathrm{th}}(\beta, n). \tag{S8}$$

Combining Eqs. (S7) and (S8), we obtain the desired result:

$$S_{\mathrm{vN}}(\hat{\rho}_n)/n = S_{\mathrm{th}}(\beta, n)/n + o(n^0) + o((N/n)^0) \tag{S9}$$

*for all Gibbs and TPQ states.* Notice that the result holds for any quantum states representing the same thermal equilibrium state of size $N$, other than the Gibbs and the TPQ states.

*Entanglement entropy.*
For a *pure* quantum state of a system of size $N$, the von Neumann entropy $S_{\mathrm{vN}}(\hat{\rho}_n)$ of its subsystem of size $n$ is a good measure of the bipartite entanglement, i.e. it well quantifies the entanglement between the subsystem and the rest of the system. This does not hold for a mixed state of size-$N$, which is a classical mixture of pure quantum states.

In our case, a TPQ state is a pure quantum state of the system of size $N$, and its $S_{\mathrm{vN}}(\hat{\rho}_n)$ safely quantifies the bipartite entanglement of the TPQ state. By contrast, a Gibbs state is a *mixed* quantum state, whose entanglement is *not* qualified by $S_{\mathrm{vN}}(\hat{\rho}_n)$. For example, the Gibbs state at infinite temperature is a maximally mixed state, whose entanglement should be zero by any measure of entanglement of mixed states, whereas $S_{\mathrm{vN}}(\hat{\rho}_n)$ takes the maximum value.

This fact clearly shows that entanglement is not an intrinsic property of thermal equilibrium states. (For more discussions, see Ref. [5].) Hence, in general, Eq. (S9) should not be understood as a property of entanglement.

---


[1] For simplicity, we exclude the first-order phase transition region, where $(\beta, N)$ cannot fully specify the equilibrium state.

[2] Yasushi Yoneta and Akira Shimizu, *Squeezed ensembles for systems with first-order phase transitions*, Phys. Rev. B **99**, 144105 (2019).

[3] In general, the condition $1 \ll n$ is necessary because otherwise the effect of the interaction Hamiltonian between the subsystem and the rest of the system would be non-negligible.

[4] When $N$ is the number of moving particles, $\hat{\rho}_n$ is the grand-canonical Gibbs state.

[5] S. Sugiura and A. Shimizu, *New Formulation of Statistical Mechanics using Thermal Pure Quantum States*, ‘Physics,Mathematics, and All that Quantum Jazz’ (edited by S. Tanaka, M. Bando and U. Gungordi), Kinki University Series on Quantum Computing: Volume 9 (2014) 245; arXiv:1312.5145.
